# Supplementary material for: Scene-Generalizable Interactive Segmentation of Radiance Fields
Source: arXiv:2308.05104 source file (2023-08-09)
Supplement: Supplementary file 1 [file fig_additional_ablation.tex]

\begin{figure*}[!t]
\centering
\includegraphics[width=0.90\linewidth]{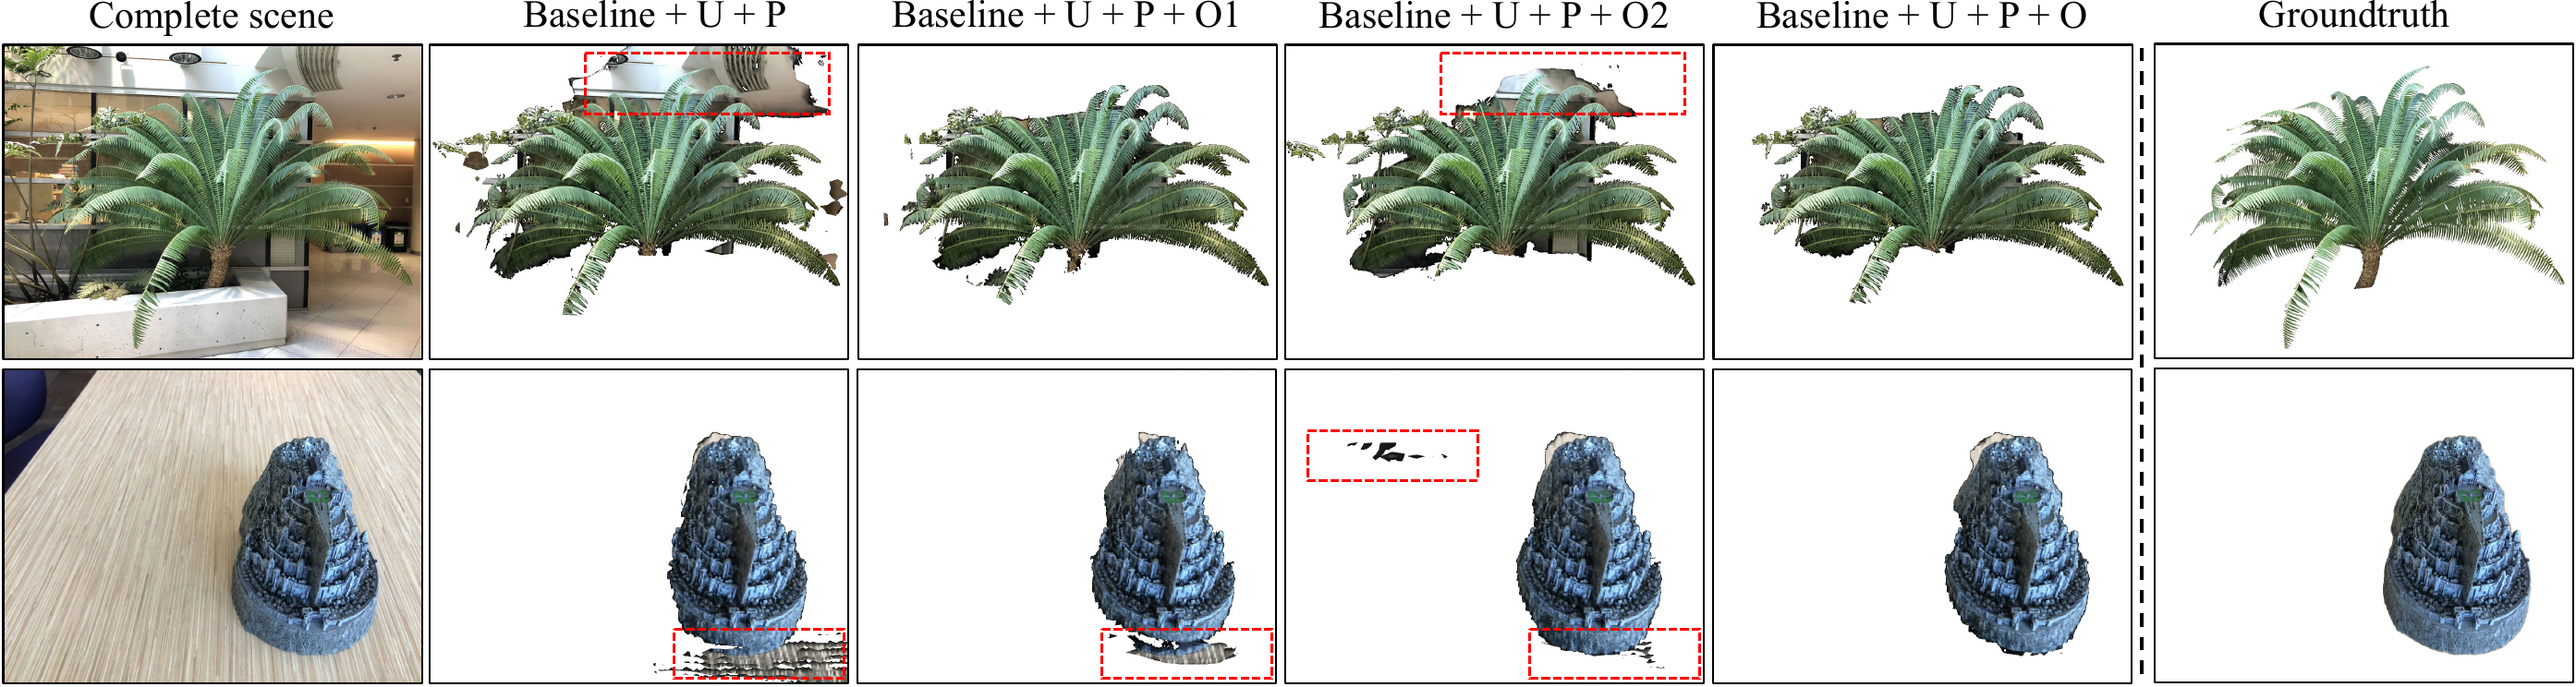}
\vspace{-8pt}
\caption{Visualization of rendering segmented foreground scenes. `U', `P', `O1', `O'and `O' denote `Uncertainty-Eliminated 3D segmentation’, `Cross-Dimension Guidance Propagation', ‘Object-Exclusive Segmentation Supervision with only $\mathcal{L}_\text{obj}^1$’ , ‘Object-Exclusive Segmentation Supervision with only $\mathcal{L}_\text{obj}^2$’ and `the total Object-Exclusive Segmentation Supervision’ respectively.}
\label{fig:addition ablation1}
% \vspace{-8pt}
\end{figure*}
