# Supplementary material for: Scene-Generalizable Interactive Segmentation of Radiance Fields
Source: arXiv:2308.05104 source file (2023-08-09)
Supplement: Supplementary file 3 [file fig_additional_co3d.tex]

% set for \usepackage{stfloats}
% \begin{figure*}[hb] 
\begin{figure*}[!t]
\centering
\includegraphics[width=0.82\linewidth]{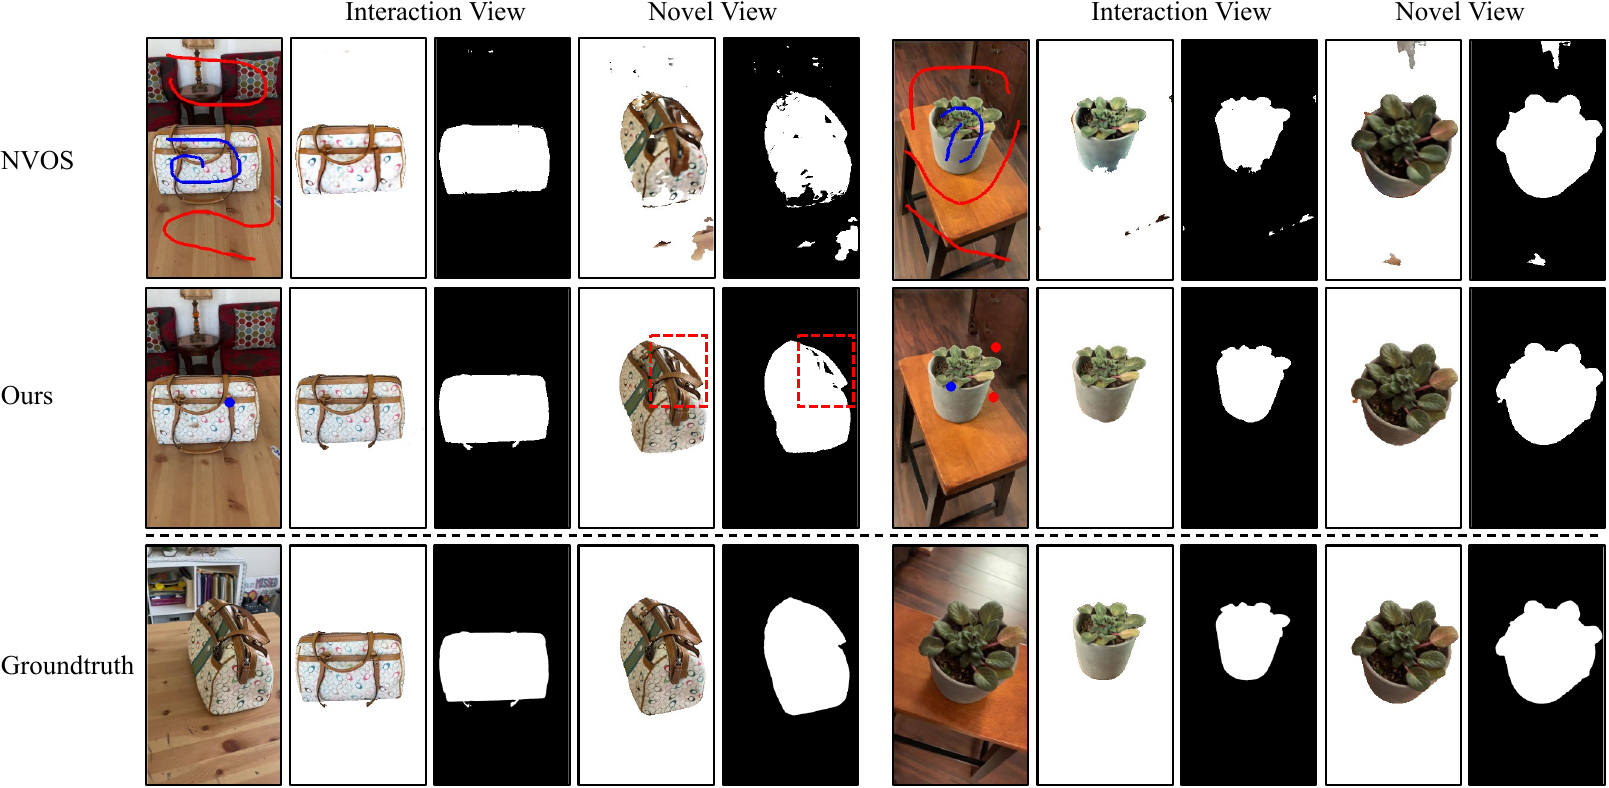}
\vspace{-10pt}
\caption{Qualitative comparison with NVOS on CO3D dataset. Our method outperforms NVOS on both cases.  As highlighted by red dashed boxes, our method even produces more precise segmentation than the groundtruth.}
\label{fig:appedix-co3d}
%\vspace{2pt}
\end{figure*}
