# Supplementary material for: Scene-Generalizable Interactive Segmentation of Radiance Fields
Source: arXiv:2308.05104 source file (2023-08-09)
Supplement: Supplementary file 4 [file fig_additional_llff.tex]

% set for \usepackage{stfloats}
% \begin{figure*}[hb] 
\begin{figure*}[!t]
\centering
\includegraphics[width=0.82\linewidth]{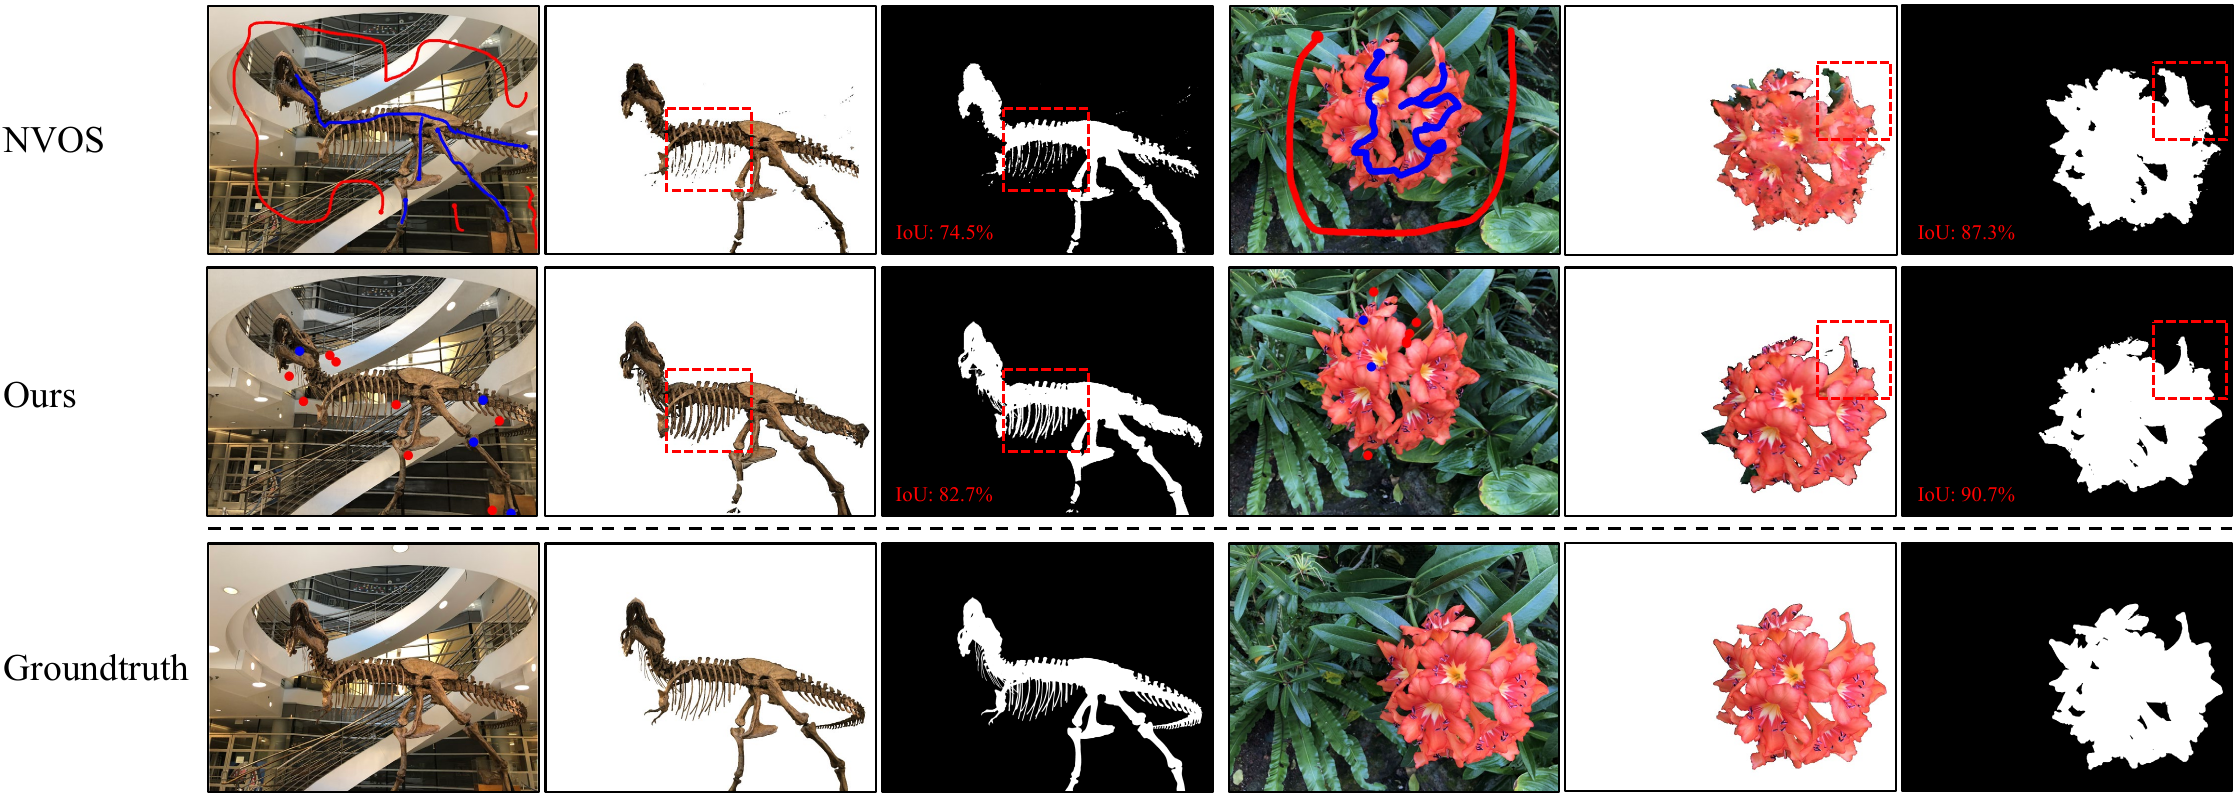}
\vspace{-10pt}
\caption{Visual Comparison with NVOS on NeRF-LLFF. The positive and negative user interactions are indicated by blue and red points, respectively. As highlighted by red dashed boxes, our method segments the rib-cage bones of T-Rex more finely.}
\label{fig:appedix-comparsion-llff}
% \vspace{-10pt}
\end{figure*}
